# Supplementary material for: Subspace Selection via DR-Submodular Maximization on Lattices
Source: arXiv:1805.07455 source file (2018-05-18)
Supplement: Supplementary file 1 [file appendix.tex]

\section{Curvatyre}
\label{sec:curvature}

\section{Matroid Constraint}
\label{sec:matroid}

We next show that greedy algorithm gives 1/2 approximation for the POS-matroid constrained submodular maximization problem.
\begin{lemma}[Fisher, Nemhauser, and Wolsey~\cite{fisher1978analysis}]
Let nonnegative numbers $\sigma_i, \rho_i$ for $i=1,2,\dots, k$ such that $\sum_{i=1}^t \sigma_{i} \le t$ and $\rho_t \le \rho_{t-1}$ for all $t = 1,2,\dots, k$ be given.
Then,
\begin{align}
  \sum_{i=1}^k \sigma_i \rho_i \le \sum_{i=1}^k \rho_i.
\end{align}
\end{lemma}
\begin{lemma}
Let $X \in S(P)$ and $x$ such that $X + x$ is admissible. Then $\|X+x\| = \|X\| + 1$.
\end{lemma}
\begin{proof}
Let $X'$ be a subspace such that $X \subsetneq X' \subset X + x$.
We need to show that $X' = X + x$.
Let $w \in \subsetneq X' \setminus X$.
Since $w \in X + x$, Lemma \ref{lemma:join} implies that there exists $y \in X$ such that $C(x,y,w)$.
This means $x \in X'$, especially, $X+x \subset X$.
\end{proof}
\begin{theorem}
Algorithm~\ref{alg:greedy} is $1/2$ approximation.
\end{theorem}
\begin{proof}
We first introduce notation.
Let $X_i$ be the $X$ in Algorithm~\ref{alg:greedy} after the $i$-the iteration.
The optimal subspace is denoted by $X^*$.
Let $x_t$ be the element chosen in the Algorithm~\ref{alg:greedy} so that $X_t = X_{t-1} + x_t$
Let 
\begin{align}
R_t = \{p \in P \mid  f(p \mid X_t) \ge f(X_{t+1}) - f(X_t), X_{t} + p \not \in  \mathcal{F}  \} \cup (X_t \setminus X_{t-1}) \setminus \bigcup_{i=1}^{t-1} R_i.
\end{align}
Let $R_k = P \setminus \bigvee_{i = 1}^{k-1} R_t$
We take $\{a_1, a_2, \dots a_k\}$ so that $X^* = (\dots(\emptyset + a_1) + a_2) \dots) + a_k$.
Let $A_l = (\dots(\emptyset + a_1) + a_2) \dots) + a_l$.
Let the set $\mathrm{OPT}(X,t)$ be $\{a_i \mid a_i \in R_t\}$.
The number $\sigma_l$ is defined as 
$\sigma_t = |\mathrm{OPT}(X,t)|$.
%\COMM{SN}{$\bigvee$はその集合を含む最小のsubspaceの意．}
Let $\rho_t = f(X_t) - f(X_{t-1})$.

We first prove that $\sigma_l$ and $\rho_t$ satisfies the conditions of the above lemma.
Notice that $X_t$ is maximal independent set in $\bigvee \left( \bigcup_{i=1}^t R_t\right)$ by the property of the algorithm \COMM{SN}{ここがまずい気がしてきた．} \COMM{SN}{(M2)を強くすれば良さそう．(M2) $X = \sum_{i=1}^k x_i$, $Y = \sum_{i=1}^{k'} y_{k'}$, $k \le k'$ ならば，$y_i \not \in X$ がとれて，$X + y_i \in \mathcal{F}$

こう定義しなおすと話がうまくいく．仮に$\sum_i^t \sigma_i > t$とすると，$X_t + a_i \in \mathcal{F}$となるが，これは$R_t$の定義に矛盾する．

uniform, partition matroidあたりは相変わらずOK．
}.
\COMM{TM}{マトロイドのランク関数を $r$ として $r(X_t + a_1 + ... + a_s) = r(X_t)$ を示せばよい（$+$ は左結合）．もしこれが成り立つなら単調性より $t = r(X_t) = r(X_t + a_1 + \cdots + a_s) \ge r(a_1 + \cdots + a_s) = s = \sum_j \sigma_j$ で従う．あやしい！ $a_1 + \cdots + a_s$ の各和が admissible とは限らないのでランクが $s$ より大きくなりうる．列を左からみていき，最適解に含まれる admissible elem なら足す，みたいなアルゴリズムを走らせる？

アルゴリズムの性質から $r(X_t + a_j) = r(X_t)$ がすべての $j \le s$ で成立することはわかっている．これに劣モジュラ性を使えば集合の場合は成り立つ．今の場合はどうか？（直感的には成り立つ気がする）
}
\COMM{SN}{いっそのことマトロイドの定義の$r$の劣モジュラ性をstrong DRに変えてしまう？(M2')は成立するので，poset matroidの拡張になっているし，$r(X_t) = r(X_t + a_1 + \cdots + a_s)$になるので上の証明もうまくいく．}
\COMM{TM}{マジすか（昼間考えたけどよくわからなかった方針です）．それでいくならとても格好良いのでぜひそうしたい．}

\COMM{SN}{
(M2') 

strong DR から劣モジュラ性が従えばOK．$f$をstrong DRな関数とする．
$X \lor Y = X + y_1 + y_2 + \dots + y_s$を取る．
\begin{align}
  f(X \lor Y) - f(X) &= \sum_{i=1}^s [f(X + y_1 + \dots + y_i) - f(X + y_1 + \dots + y_{i-1})]\\
  &\le \sum_{i=1}^s [f((X \land Y) + y_1 + y_2 + \dots + y_i) - f((X \land Y) + y_1 + y_2 + \dots + y_{i-1})]
\end{align}
不等式はstrong DR．
$y_1 + y_2 + \dots + y_i \subset Y$に注意してモジュラ性を使うと，$(X \land Y) + y_1 + y_2 + \dots + y_i = (X + y_1 + \dots + y_i) \land Y$．とくに$i=s$のとき$Y$になる．あとはtelescoping sumで最右辺が$f(Y) - f(X \land Y)$になる．
$X \land Y$に足すのがadmissibleなのは，モジュラ性を使うのとdiamond isomorphismで行ける.

マトロイドランクの方：
\begin{align}
r(X_t + a_1 + a_2 + \dots a_s) &= r(X_t) + \sum_{i=1}^s [r(X_t + a_1 + \dots + a_i) - r(X_t + a_1 + \dots + a_{i-1})]\\
&\le r(X_t) + \sum_{i=1}^s [r(X_t  + a_i) - r(X_t)] = r(X_t)
\end{align}
不等式はstrong DR．逆向き不等式は単調性．
}
\COMM{TM}{あー，納得しました (weak だと思ってた)．こっちでもまあよいかも．weak でも admissibility はいりますよね．}
\COMM{SN}{$r(a_1 + \dots + a_s) = s$の部分だったら，ここのadmissibilityはweakでも要ります．}
\COMM{TM}{$Y_j$ を $x_j$ 手前までのすべての join irreducibles とする．$\tau_j = r(Y_j)$ とおき，$\rho_j = \tau_{j+1} - \tau_j$ で定義する．このとき $\tau_j \le j$ が従う．

いま任意に $X \lor X^* = X + x_1^* + \cdots + x_m^*$ なる $x_1^*, \ldots, x_m^*$ たちを固定する．そして
\begin{align}
f(X \lor X^*) - f(X) 
&= \sum_j f(X + x_1^* + \cdots + x_j^*) - f(X_1 + x_1^* + \cdots + x_{j-1}^*) \\
&= \sum_j \sum_p f(X_i + y_p^*) - f(X_i) 
\end{align}
ただし $p$ の総和範囲は $j$ 番目のブロックを走る．ブロック内の要素数は $\rho_j$ 個しか存在しない．

$y_p^*$ が $X_i$ に足せることはマトロイド公理で保証する必要がある．$y_p^*$ は $y_p^* \le \tilde x_p^*$ for some $x_p^*$．
}
\COMM{TM}{supermatroid (Dunstan, Ingleton, Welsh'72) なる概念がある．

$\mathcal{I}$ が supermatroid if $0 \in \mathcal{I}$; $x \le y$, $y \in \mathcal{I}$ then $x \in \mathcal{I}$; 任意の $x$ について $y \in I_x \cap \mathcal{I}$ の極大元は同じ高さをもつ

strong supermatroid if $r(x) \le r(y) \le r(x)+1$ if $y$ covers $x$; $x, x'$ covers $y$, $z$ covers $x, x'$, $r(y) = r(x) = r(x')$ then $r(y) = r(z)$.

unit incrementは仮定が必要で，ないと反例があるそうな．

strong supermatroid を仮定すると $r(X + a_1 + \cdots + a_k) = r(X)$ が出る: $X$ を $X + a_1$, $X + a_2$ がそれぞれ cover $X + a_1 + a_2$ に cover されるので．
$r(a_1 + \cdots + a_k)$ について join irreducible な要素たちを相対的な順序関係を変えずに「下に下ろす」と admissible に足せるので OK．単調減少性は unit increment から出す．
}
%The subspace $\bigvee \left(\bigcup_{i=1}^{t} \mathrm{OPT}(X,i) \right)$ is independent set.
%Since the maximal independent set have the same cardinality , we have 
%\begin{align}
%\sum_{i=1}^t \sigma_i = \|X^*  \land \bigvee_{i=1}^l R_t  \| \le \|X_t\| = t.
%\end{align}
Let $w \in \mathrm{cl}(x_{i+1} \mid X_i)$ and $w' \le w$ such that $X_{i-1} + w'$ is admissible.
Since $X_i + w = X_{i+1} \in \mathcal{F}$, the subspace $X_{i-1} + w' \subseteq X_i + w$ is independent owing to (M1).
Hence, by the greediness of the algorithm, $f(w \mid X_{i-1}) \le \rho_i$.
By DR-submodularity, we have $\rho_{i+1} \le \rho_{i}$.

By the monotonicity,
\begin{align}
  f(X^*) &\le f(X^* \lor X) \le f(X) + \sum_{i=1}^k (f(X \lor A_i) - f(X \lor A_{i-1}))\\
  &= f(X) + \sum_{t=1}^k \sum_{a_i \in \mathrm{OPT}(X,t)} (f(X \lor A_i) - f(X \lor A_{i-1}))\\
  &\le^{(*)} f(X) + \sum_{t=1}^k \sum_{a_i \in \mathrm{OPT}(X,t)} (f(X_i) - f(X_{i-1}))
  = f(X) + \sum_{t=1}^k \sigma_t \rho_t\\
  &\le^{(**)} f(X)  \sum_{t=1}^k \rho_t = 2f(X).
\end{align}
In (*), we used the following argument.
We first prove that, for any $a_i \in \mathrm{OPT}(X,t)$, there exists $a' \le a_i$ such that $X_{t-1} + a' \in \mathcal{F}$.
\COMM{SN}{これが成立すると思ったけどダメっぽい．今の(M3)だとうまくいかない．}
Since $X_t + a_i$ is admissible, one of the following cases occurs.
First, $x_t \le a_i$ and there is no element between $x_t$ and $a_i$.
In this case, $X_{t-1} + x_t = X_t \in \mathcal{F}$.
Second, $X_{t-1} + a_i$ is admissible.
Since $a_i \not \in \mathrm{OPT}(X,t)$, 
In (**), we used the lemma above.
\COMM{TM}{
diamond isomorphism で $X^* = X \land X^* + y_1^* + \cdots + y_m^*$ をとる ($y_j^* \le x_j^*$; 本当？)．$X \land X^*$ はマトロイド独立集合なので各 $y_j^*$ たちは全部 unit increment を与える．

% 最後の部分も多分正しい．$f(X + a_1 + \cdots + a_p) - f(X + a_1 + \cdots + a_{p-1})$ に対して weak DR submodularity を使い上から $f(X_i + b_p) - f(X_i)$ で抑える．ただし $b_p \le \tilde a_p$, $X + .... + a_p = X + ... + \tilde a_p$．
}
\end{proof}
